# Supplementary material for: Efficient first principles based modeling via machine learning: from simple representations to high entropy materials
Source: arXiv:2403.15579 ancillary file (2024-03-22)
Supplement: Supplementary file 1 [file ESI.pdf]

# Supplemental Material for *Efficient first principles based modeling via machine learning: from simple representations to high entropy materials*

Kangming Li,[1,*] Kamal Choudhary,[2] Brian DeCost,[2] Michael Greenwood,[3] and Jason Hattrick-Simpers[1,4,5,6,†]

[1] *Department of Materials Science and Engineering, University of Toronto, 27 King's College Cir, Toronto, ON, Canada.*
[2] *Material Measurement Laboratory, National Institute of Standards and Technology, 100 Bureau Dr, Gaithersburg, MD, USA.*
[3] *Canmet MATERIALS, Natural Resources Canada, 183 Longwood Road south, Hamilton, ON, Canada.*
[4] *Acceleration Consortium, University of Toronto. 80 St George St, Toronto, ON M5S 3H6.*
[5] *Vector Institute for Artificial Intelligence, 661 University Ave, Toronto, ON, Canada.*
[6] *Schwartz Reisman Institute for Technology and Society, 101 College St, Toronto, ON, Canada.*

Supplementary Table I. Number of structures as functions of number of atoms and number of elements.

| # atoms | # elements | | | | | |
|---|---|---|---|---|---|---|
| | 2 | 3 | 4 | 5 | 6 | 7 |
| 2 | 40 | 0 | 0 | 0 | 0 | 0 |
| 3 | 252 | 210 | 0 | 0 | 0 | 0 |
| 4 | 797 | 4342 | 2633 | 0 | 0 | 0 |
| 5 | 745 | 2643 | 2669 | 108 | 0 | 0 |
| 6 | 2707 | 11933 | 18402 | 3000 | 0 | 0 |
| 7 | 0 | 0 | 0 | 0 | 0 | 854 |
| 8 | 434 | 2970 | 5790 | 3049 | 3132 | 2865 |
| 27 | 486 | 2505 | 3021 | 3077 | 783 | 56 |
| 64 | 229 | 797 | 521 | 1641 | 400 | 108 |
| 125 | 0 | 0 | 0 | 0 | 0 | 598 |

* kangming.li@utoronto.ca
† jason.hattrick.simpers@utoronto.ca

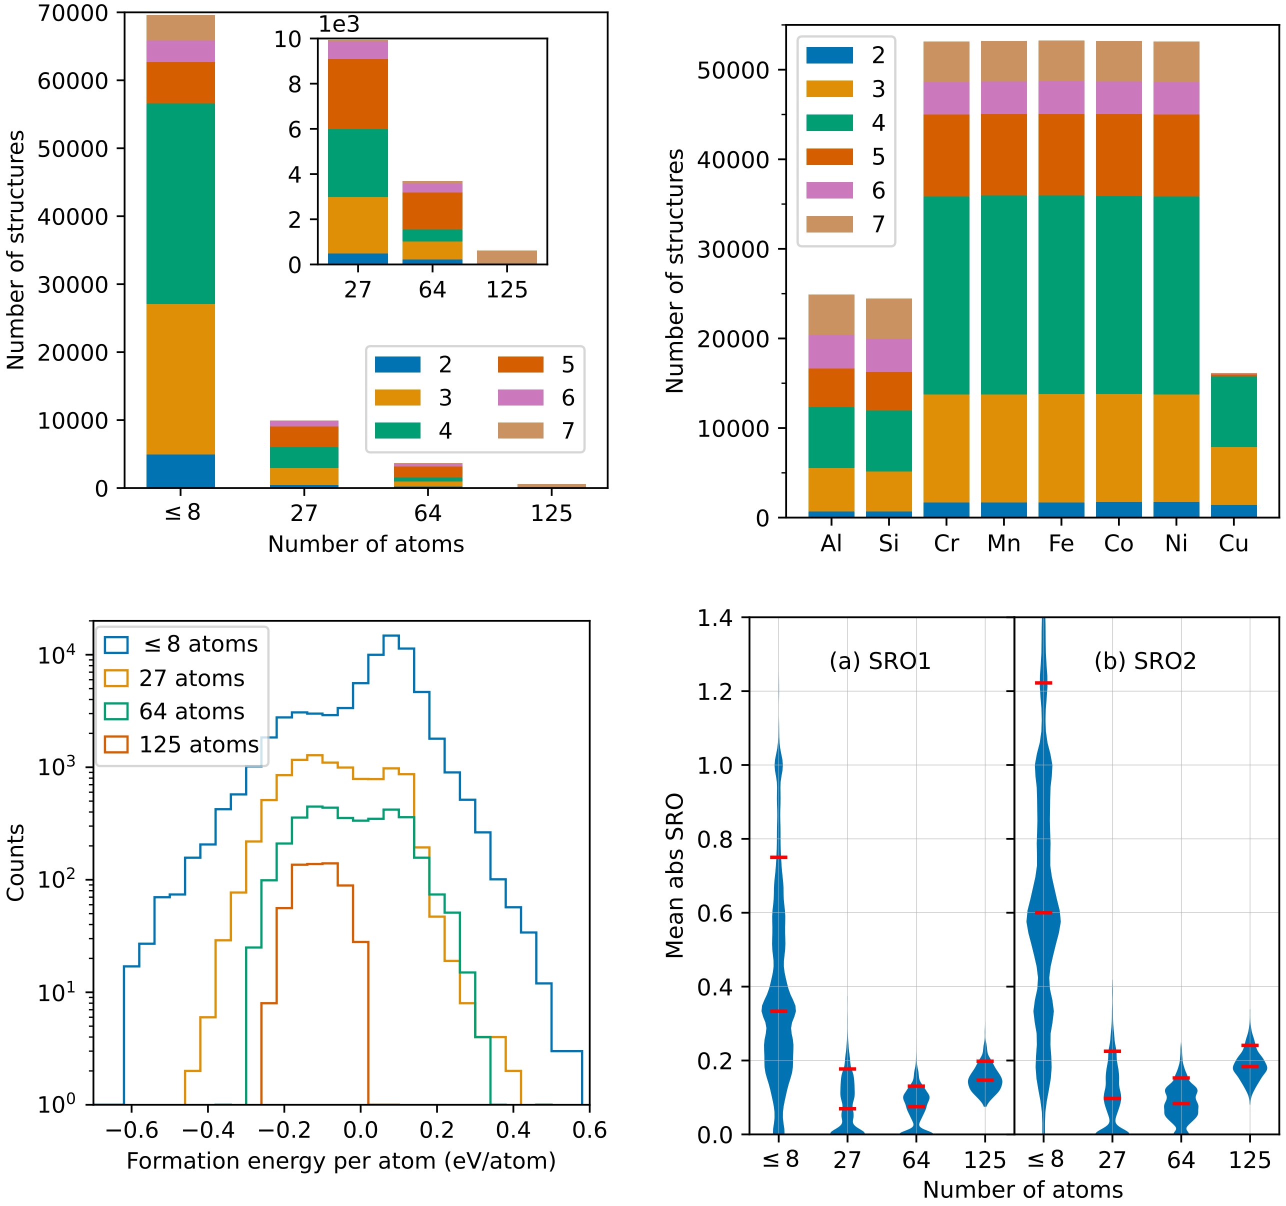


Supplementary Figure 1. Distribution of structures as functions of system size (upper left), element (upper right), formation energy (lower left), and SROs (lower right). Upper left panel: The legend indicates the number of components, and the inset is an enlarged view for SQSs. Upper right panel: The legend indicates the number of components, and the X axis indicates the element contained in the structures. Lower right panel: The violin plot indicates the distribution of structures as functions of SRO and system size for the first and second coordination shells.

Supplementary Table II. Hyperparameter search results. We perform a hyperparameter grid search based on 5-fold cross validations within the in-distribution training set. The ranges of hyperparameter values, the best values, and the values used in the paper are reported. The comment row mentions the best MAE and the current MAE, which are practically the same.

| Model | Hyperparameters | Value range | Best | Used in paper |
|---|---|---|---|---|
| Random forest | bootstrap | [True, False] | False | False |
| | max_depth | [5, 10, 15, 20, None] | None | None |
| | max_features | [0.1, 0.2, 0.3, 0.45] | 0.3 | 0.3 |
| | n_estimators | [50, 100, 150, 200] | 200 | 100 |
| Comment | Best vs. current MAE: 15.9 vs. 16.0 meV/atom | | | |
| | | | | |
| XGBoost | n_estimators | [500, 1000, 2000, 3000] | 2000 | 500 |
| | learning_rate | [0.1, 0.2, 0.3, 0.4] | 0.2 | 0.4 |
| | colsample_bytree | [0.3, 0.5, 0.7, 0.9] | 0.9 | 0.5 |
| | colsample_bylevel | [0.3, 0.5, 0.7, 0.9] | 0.3 | 0.7 |
| | num_parallel_tree | [4, 6, 8, 10] | 10 | 6 |
| Comment | Best vs. current MAE: 13.6 vs. 14.4 meV/atom | | | |
